# Supplementary material for: Reducing the time-step errors in diffusion Monte Carlo
Source: arXiv:2312.01526 ancillary file (2024-03-15)
Supplement: Supplementary file 1 [file si.pdf]

# Supplementary Material for Reducing the time-step errors in diffusion Monte Carlo

Tyler A. Anderson<sup>a,1</sup> Manolo C. Per<sup>b,2</sup> and C. J. Umrigar<sup>c1</sup>

<sup>1</sup>*Laboratory of Atomic and Solid State Physics,  
Cornell University, Ithaca, NY 14853.*

<sup>2</sup>*CSIRO Data61,  
Clayton, VIC 3168, Australia.*

## S1. TIME-STEP ERROR OF THE TOTAL ENERGY FOR ALL-ELECTRON SYSTEMS

In Fig. S1 we show the time-step errors for three all-electron (no pseudopotential) systems - Be, Ne and N<sub>2</sub> - using the reweighting factor of Eq. 13. We employ Slater rather than Gaussian basis functions and impose the electron-nucleus cusp conditions. Specifically, we used the CVB1 Slater basis<sup>1</sup> and 2 CSFs (4 determinants) for Be, the CVB2 Slater basis<sup>1</sup> and 442 CSFs (12,898 determinants) for Ne, and the CVB2 Slater basis<sup>1</sup> and 1880 CSFs (12,138 determinants) for N<sub>2</sub>. 7<sup>th</sup>-order electron-electron-nucleus Jastrow factors<sup>2</sup> were used for all the systems. For the new reweighting scheme, we show curves both for values of  $c$  obtained from Eq. 15 (shown in Table S1) as well as for some other values of  $c$ . It is clear that the new reweighting along with the  $c$  values from Eq. 15 and  $k = 15.51$  give much flatter curves than the naive and the UNR93 reweighting. The flattest curves for all three systems are remarkably flat and correspond to using  $k = 12$  in Eq. 15. Since the use of pseudopotentials makes QMC calculations much more efficient, the new reweighting factor was originally developed and tested on pseudopotential systems only. So, it is remarkable that the reduction in the time-step errors are even greater for the all-electron systems than for the pseudopotential systems.

TABLE S1. Autocorrelation times in Monte Carlo steps for  $\tau = 0.01 \text{ Ha}^{-1}$  and  $c$  according to Eq. 15 for the all-electron systems studied. For these systems, flatter curves can be obtained by using  $k = 12$  rather than  $k = 15.51$  as can be seen from Fig. S1.

| System                        | $T_{\text{corr}}$ | $c$ using $k=15.51$ | $c$ using $k=12$ |
|-------------------------------|-------------------|---------------------|------------------|
| Be CVB1, 2-CSF                | 8.04              | 5.85                | 4.52             |
| Be CVB2, 100-CSF              | 6.83              | 6.42                | 4.97             |
| Ne CVB2, 442-CSF              | 2.44              | 12.92               | 10.              |
| N <sub>2</sub> CVB2, 1880-CSF | 4.06              | 8.87                | 6.86             |

We have argued in the text that the new reweighting scheme does not change the slope of the energy versus  $\tau$  curve at  $\tau = 0$ . However some of the plots in the main paper and the supplementary material appear to contradict this. The resolution of this seeming contradiction is that although the slope at  $\tau = 0$

<sup>a</sup> taa65@cornell.edu

<sup>b</sup> Manolo.Per@data61.csiro.au

<sup>c</sup> CyrusUmrigar@cornell.edu

is unchanged, it does change rather rapidly for small  $\tau$  particularly for large values of  $c$  in Eqs. 13 and 14. It is apparent that this must happen because for  $c \rightarrow \infty$  the energy must be the fixed-node DMC energy at  $\tau = 0$ , but, it must equal the VMC energy for all other values of  $\tau$ . To make this plausible, we show in Fig. S1(b) the energy versus  $\tau$  curves for Be using a finer scale than in Fig. S1(a).

Next we demonstrate that the difference in the time-step error resulting from using Eq. 13 or Eq. 14 is minor compared to the time-step error of the naive and UNR93 reweighting schemes. We do this by showing in Fig. S2 the energy versus  $\tau$  curves for a Be atom using the CVB2 basis and 100 CSFs (764

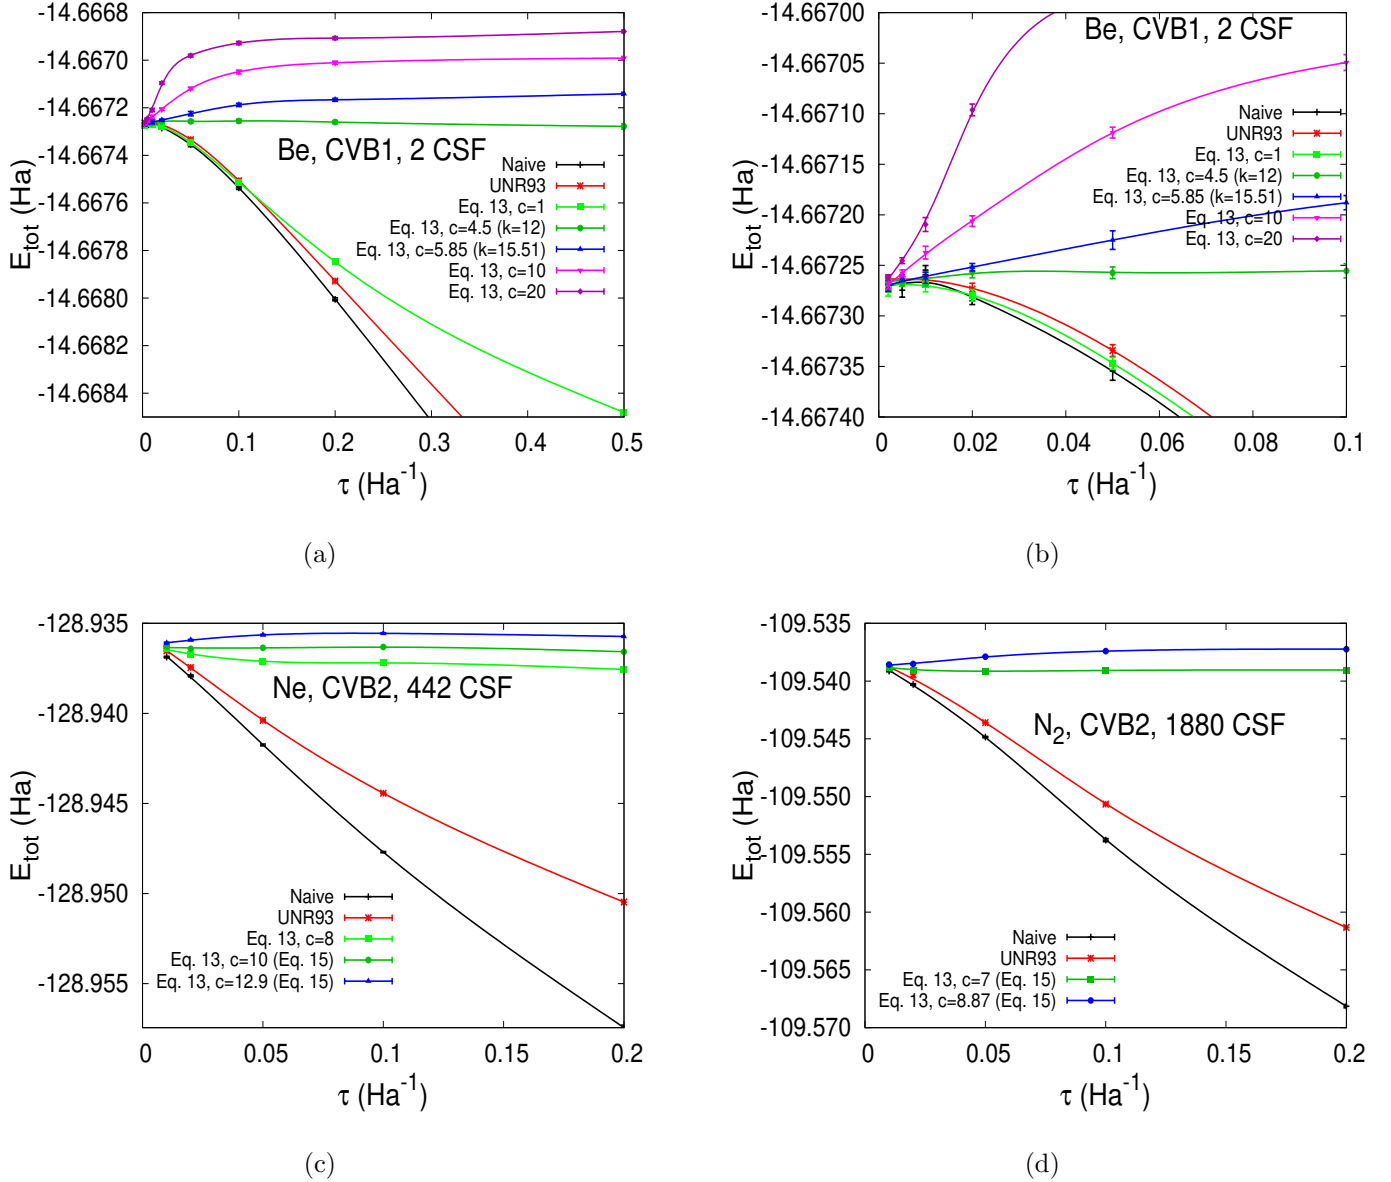

FIG. S1. Comparison of time-step errors of the total energy for the naive, UNR93 and new reweighting factors for Be, Ne and N<sub>2</sub>. The new reweighting curves are shown for a few different values of  $c$ , including the values prescribed by Eq. 15 for  $k = 15.51$  (blue curves) and  $k = 12$  (web-green curves). Fig. S1(b) is the same as Fig. S1(a) but on a finer scale. The curves for  $c = 1$ ,  $c = 10$  and  $c = 20$  for Be are plotted simply to demonstrate that in the  $c \rightarrow 0$  the curve tends to the one for the naive reweighting, and that in the  $c \rightarrow \infty$  limit the energy tends to the VMC energy for all values of  $\tau$  except  $\tau = 0$ .

determinants). Note that Fig. S2 employs a finer scale on the energy axis than the Be curves in Fig. S1 because the improved wave function has a smaller time-step error for all reweighting schemes. We note that for this system (as well as for other all-electron systems we have studied but not presented in this paper) the curve resulting from using Eq. 13 is even flatter than that from Eq. 14.

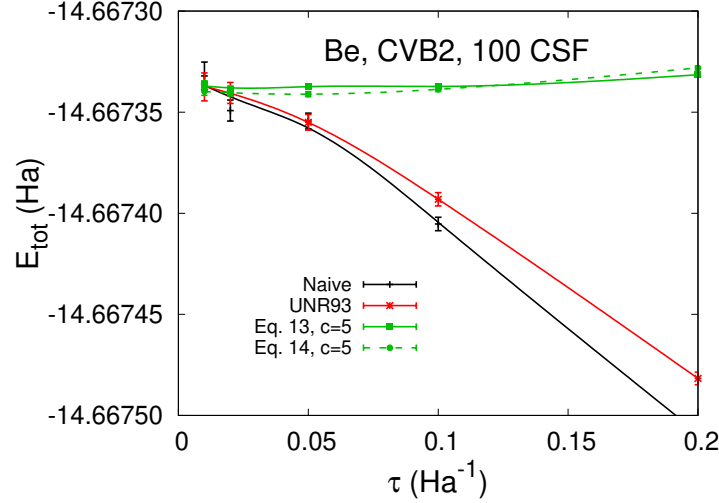

FIG. S2. Comparison of time-step errors of the total energy for the naive, UNR93 and new reweighting factors for Be using the CVB2 basis and 100 CSFs. The reweighting factors of both Eq. 13 and Eq. 14 give very flat curves, and Eq. 13 gives an even flatter curve than Eq. 14.

## S2. TIME-STEP ERROR OF KINETIC ENERGY

Here we show the reduction in the time-step error of the kinetic energy resulting from our new reweighting factor. The improvement in the time-step error is not as large as the improvement for the total energy shown in the main text. In the case of 1-CSF carbon, the new reweighting in fact gives a larger time-step error than the naive and the UNR93 reweighting factors. However, this is simply because the naive and UNR93 reweighting factors by chance happen to give a very small time step error for this particular system. This is evidenced by the fact that for  $\tau = 0.5$  the naive reweighting has a 7 mHa error for 29-CSF carbon but only a 1 mHa error for 1-CSF carbon.

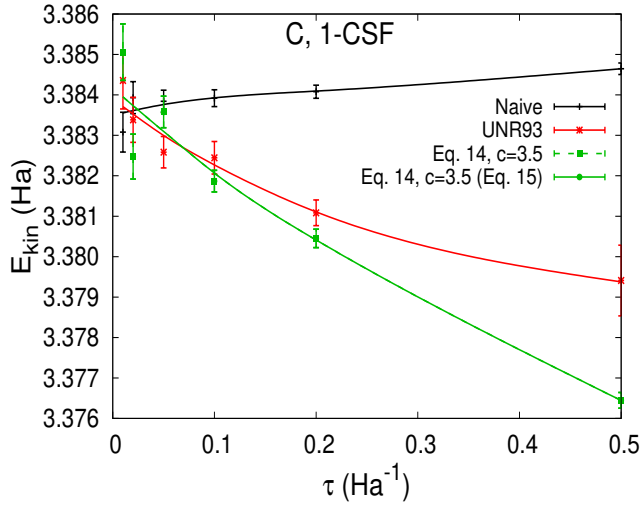

(a)

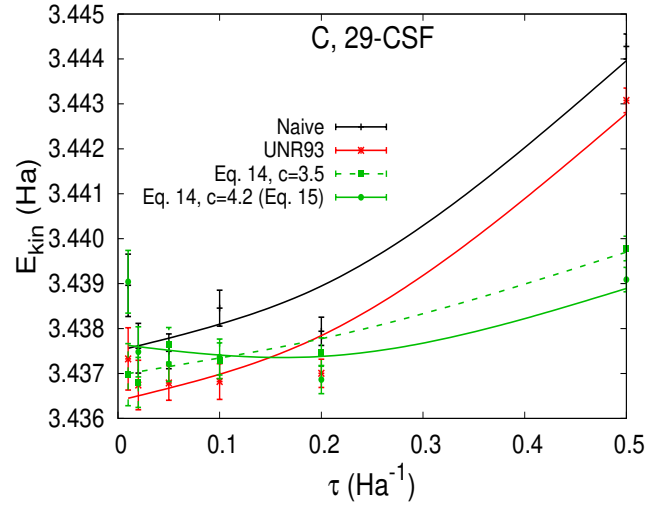

(b)

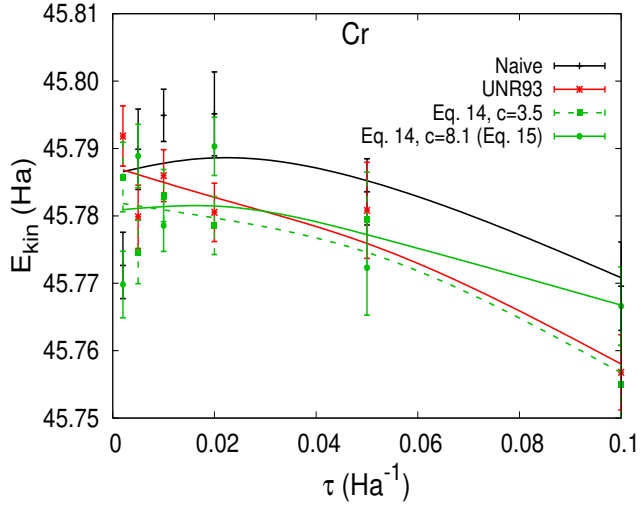

(c)

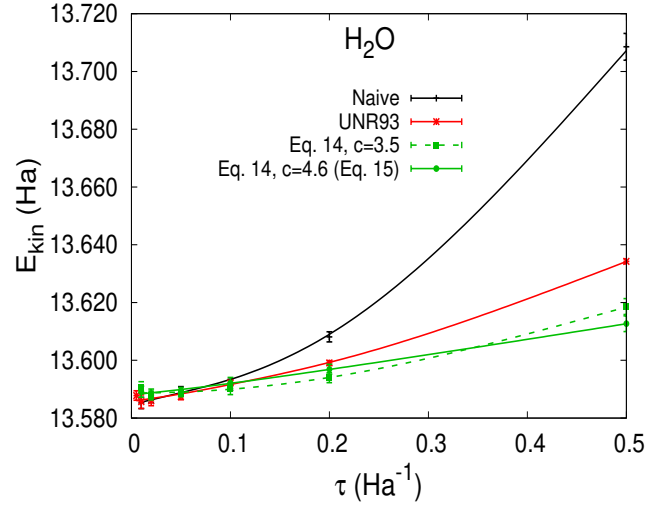

(d)

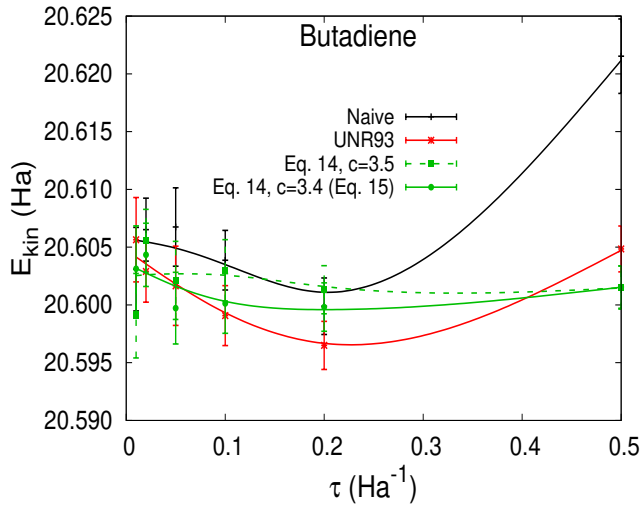

(e)

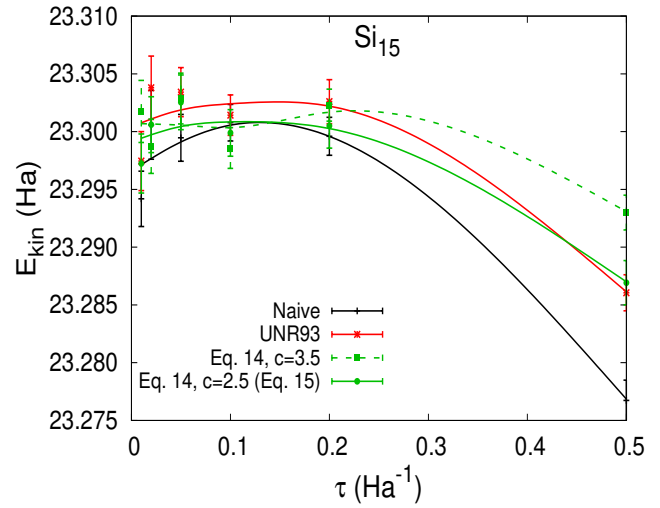

(f)

FIG. S3. Comparison of time-step errors of the total kinetic for the naive, UNR93 and new reweighting factors.

- 
- <sup>1</sup> I. Ema, J. M. Garcia de la Vega, G. Ramirez, R. Lopez, J. Fernandez Rico, H. Meissner and J. Paldus, J. Comput. Chem. **24**, 859 (2003).
- <sup>2</sup> A. D. Güclu, G. S. Jeon, C. J. Umrigar, and J. K. Jain, Phys. Rev. B **72**, 205327 (2005), see Eqs. 3 and 5.
